# Supplementary material for: RedLight-VLA: Models for traffic-rule grounding and behavioral emphasis in driving policies
Source: arXiv:2608.28656 source file (2026-08-21)
Supplement: Supplementary file 1 [file 08_appendix.tex]

\appendix
\section{Additional Controls and Metric Definitions}
\label{sec:appendix}

\paragraph{Auxiliary readout controls.}
Table~\ref{tab:readout} compares auxiliary readout designs that use the same
supervision targets. \textbf{AUX-pre} reads a soft tokenizer that
cross-attends the vision embeddings before the LLM. \textbf{AUX-pool} reads the
mean-pooled post-LLM sequence with no reserved tokens. \textbf{AUX} reads
reserved post-LLM slots. \textbf{AUX-text} decodes the rule state as a short
text target through the language head in the style of
EMMA~\cite{hwang2024emma}. The variants differ in representation source,
aggregation, and whether reserved slots are present. The table is therefore an
architectural comparison, not a placement-only ablation.

\begin{table}[!ht]
\centering
\caption{\textbf{Alternative auxiliary readout designs.} All rows use the
same perception-derived supervision targets. The incomplete cells remain
placeholders pending matched evaluations.}
\label{tab:readout}
\small
\begin{tabular}{lcccc}
\toprule
Condition & TL ADE@3s & TL FDE@3s & TL color acc. & Stop-line dist.\ MAE (m) \\
\midrule
AUX-pre            & \placeholder{--} & \placeholder{--} & \placeholder{--} & \placeholder{--} \\
AUX-pool           & \placeholder{--} & \placeholder{--} & \placeholder{--} & \placeholder{--} \\
Full (ours)        & 0.247 & 0.897 & \placeholder{--} & \placeholder{--} \\
AUX-text (stretch) & \placeholder{--} & \placeholder{--} & \placeholder{--} & \placeholder{--} \\
\bottomrule
\end{tabular}
\end{table}

\paragraph{Behavioral-reweighting controls.}
\textbf{BR-naive} uses one trigger and applies a uniform weight whenever any
$|a_t|>2\,\text{m/s}^2$, at the same $w_{\max}$. \textbf{BR-resample}
oversamples triggered frames in the dataloader at a matched effective rate.
Both controls use the same backbone and reporting buckets as BR.

\paragraph{Rule-compliance metric definitions.}
\label{sec:rule_metrics}
Sliced ADE can improve when a model brakes more often near intersections, even
if the response is not conditioned correctly on the light state. We therefore
report three open-loop rule-compliance proxies on the TL slice, following the
rule-aware scoring motivation of the nuPlan/NAVSIM PDM-score
line~\cite{caesar2021nuplan,dauner2024navsim,li2024hydramdp}.

The \emph{red-light stop-line overshoot rate} is the fraction of red-light
frames whose predicted trajectory crosses the perception stop line within the
horizon while the ground truth does not. The \emph{green-light false-stop
rate} is the fraction of green-light frames where predicted speed drops below
$v_{\text{stop}}=1.0\,$m/s while the ground truth proceeds. The
\emph{stop-line velocity error} is $|\hat v-v_{\mathrm{GT}}|$ at the
ground-truth stop-line crossing or minimum-distance time.

These metrics are computed from tensors already present in the evaluation loop.
They complement TL-sliced ADE/FDE but remain open-loop proxies rather than a
closed-loop rule-compliance evaluation.

\paragraph{Kinematic--rule overlap.}
Figure~\ref{fig:joint} crosses the behavioral-trigger state with TL relevance.
The resulting distribution is a descriptive property of the training data. It
can motivate an interaction experiment, but it does not establish that BR and
AUX are complementary.

\begin{figure}[!ht]
\centering
\fbox{\parbox{0.55\linewidth}{\centering \vspace{2mm}
\emph{2$\times$2 (or 2$\times$3) heatmap placeholder:}\\
training-frame fractions over \{kinematic trigger: DCCL / ACCL / none\}
$\times$ \{rule event: TL-relevant / none\}
\vspace{2mm}}}
\caption{\textbf{Kinematic$\times$rule joint coverage.} Training-frame
fractions are grouped by behavioral-trigger state and TL relevance. This is a
descriptive data diagnostic; interaction must be evaluated from model results.}
\label{fig:joint}
\end{figure}

% Before submission: replace the heatmap placeholder with the offline profiling
% output and report raw counts, percentages, and the denominator.

\paragraph{Gradient-share diagnostic.}
Table~\ref{tab:gradshare} is reserved for the planned comparison of gradient
share before and after reweighting. The final statistic must use the same
held-out examples in both conditions and state the differentiated parameter
subset, per-example loss, aggregation rule, and uncertainty procedure.

\begin{table}[!ht]
\centering
\caption{\textbf{Gradient share before and after reweighting.} Values remain
placeholders until the diagnostic definition and matched evaluation are
finalized.}
\label{tab:gradshare}
\small
\begin{tabular}{lcc}
\toprule
Bucket & Baseline (\%) & BR (\%) \\
\midrule
Constant     & \placeholder{--} & \placeholder{--} \\
Decelerating & \placeholder{--} & \placeholder{--} \\
Hard brake   & \placeholder{--} & \placeholder{--} \\
Launch       & \placeholder{--} & \placeholder{--} \\
\bottomrule
\end{tabular}
\end{table}

%============================================================
